# Supplementary material for: Agentic Coding Needs Proactivity, Not Just Autonomy
Source: arXiv:2605.06717 source file (2026-05-07)
Supplement: Supplementary file 1 [file appendix.tex]

\DoToC

\section{An Illustrative Day in the Life}
\label{app:walkthrough}

We move the day in the life walkthrough into the appendix to mark it explicitly as illustrative rather than as a result. It exists to make Algorithm~\ref{alg:proact} easier to read, not to claim measured validation of \ours{}. Each scenario notes the level engaged and the responsible component from Section~\ref{sec: proact}.

\paragraph{07:30. Level 2, scheduled.} Before the developer opens the laptop, a nightly Level 2 routine has run. It pulled the top three bugs from Linear, attempted fixes on two, and opened draft pull requests. A third issue was too ambiguous, so the agent drafted a clarifying comment instead. The morning briefing in the inbox reads: ``2 draft pull requests ready for review. 1 issue needs clarification. Test coverage at 81 percent, down from 83 percent last week.''

\paragraph{09:15. Level 3, situation aware.} The developer is in feature work on branch \texttt{feature/payments}. C1 detects a teammate's pull request merged 10 minutes ago that changes the payments API schema; it cross references Jira and finds the developer's ticket depends on that API; it scans Slack and finds a thread the developer was not tagged in. C2 estimates that the cost of staying silent now exceeds the cost of interrupting because the sprint ends Friday. C3 routes the action to an informational alert: ``Sarah's pull request changed the payments response format. Your branch calls this endpoint in 3 places. Sprint ends Friday. Diff attached.'' The developer taps ``Show me'' and sees the relevant code highlighted.

\paragraph{11:00. Level 2, event triggered.} Continuous integration fails on a push. A webhook routine analyzes the failure logs, identifies a known flaky test in \texttt{auth\_integration\_test.go}, and posts a comment: ``Known flaky test. Pipeline restarted. No action needed.''

\paragraph{14:00. Level 3, silence.} The agent detects a minor code style inconsistency in a teammate's pull request. C2 evaluates: the developer is in a focused coding session (no buffer switches in 45 minutes, steady commit cadence); the finding is low severity; the developer has historically dismissed style only findings during afternoon focus blocks. C3 defers the item to the weekly digest. This is the proactive behavior Level 2 cannot produce: the decision not to act.

\paragraph{16:30. Level 3, delegate.} C1 notices that three dependencies in \texttt{package.json} have backward compatible patch updates available, with passing continuous integration in the upstream repositories. C3 posts a delegate item: ``3 patch updates available. All backward compatible. Open a pull request and run your test suite?'' The developer taps ``Delegate.'' The agent handles the rest.

\paragraph{18:00. Level 2, scheduled.} An end of day routine scans the day's merged pull requests for documentation that references changed APIs, flags two stale documentation pages, and opens update pull requests. The developer will see these in tomorrow's morning briefing.

\paragraph{Discussion.}
The pattern is consistent across the day. Level 2 handles the predictable, repeatable background work. Level 3 handles the unpredictable, context dependent intelligence that connects events across silos and chooses when to show an insight or remain silent. Neither level alone is sufficient. The illustrative scenarios are coding analogues of the PARE Bench scenarios in \citet{nathani2026proactive} and were constructed by hand for this paper.

\section{Future Directions}
\label{app: future}

\paragraph{Coding focused proactive benchmark.}
Section~\ref{sec:op3} called for a public benchmark that combines suggestion, clarification, and an active user simulator. The scenario suite of Section~\ref{sec:pare-coding} is intended as the seed.

\paragraph{Personalized policy learning.}
The threshold $\tau$ in Algorithm~\ref{alg:proact} should be developer specific and time varying. The reward inference of \citet{lin2022inferringrewards} and the joint productivity, proactivity, personalization training of \citet{sun2025trainingproactivepersonalizedllm} are natural starting points.

\paragraph{Privacy and on device inference.}
A Level 3 agent ingests behavioral signals (buffer edits, dwell time, typing cadence) that are sensitive. On device relevance modeling, scoped MCP connectors, and a transparent activity log are required defaults.

\paragraph{Team scope.}
Many of the highest value proactive moments are inherently across developers (the example in Section~\ref{sec: prob_form} involves a teammate's pull request affecting the developer's branch). Extending \ours{} to model teams rather than individuals is a natural next step.

\section{Limitations}
\label{app: limitation}

\paragraph{Position paper, not deployment paper.}
The architecture, the algorithm, and the metric definitions in this paper have not been validated on a deployed system. The day in the life walkthrough in Appendix~\ref{app:walkthrough} is constructed by hand. Section~\ref{sec: analysis} states the studies that would change this.

\paragraph{Vendor capabilities are moving targets.}
The audit reflects vendor documentation at the audit date. Cursor Automations and Claude Code Routines in particular have evolved across 2025 and 2026 and will continue to evolve.

\paragraph{Audit subjectivity.}
The criteria O1 through O5 are practical rather than mathematical. The boundary between partial and full satisfaction of cross context observation requires judgment. We have erred on the side of the vendor's own claims.

\paragraph{Simulation gap.}
The simulated developer in Section~\ref{sec:pare-coding} is a language model conditioned on a profile. Real developer behavior diverges from simulated behavior in the long tail \citep{sun2025trainingproactivepersonalizedllm,zhou2026tomswe}.

\paragraph{Interruption cost extrapolation.}
\citet{meyer2024breakingflow} measure the cost of in person and real-time interruptions during software engineering activities. Whether those findings carry over to later agent messages should be measured, not assumed.

\section{Implementation Notes}
\label{app: tech_details}

\paragraph{Connector layer.}
\ours{} consumes events through MCP connectors for code (repository, branch state, diffs, test results), project (Jira, Linear), communication (Slack, pull request comments), infrastructure (continuous integration, deployment logs), and developer behavior (buffer activity, dwell time). Each connector carries scoped credentials.

\paragraph{Inbox interface.}
The reference inbox follows three established design points: the agent inbox of \citet{langchain_ambient2025,langchain_agents_from_scratch2025}, the code inbox of Uber~\citep{uber_codeinbox2026}, and the desktop application of \citet{claude_cowork2026}.

\paragraph{Relevance and timing model.}
The reference implementation maintains a per developer Bayesian preference model, updated via implicit signals (delegation latency, dismissal patterns, edits after a message) and explicit thumbs and dismiss actions. Active Inference~\citep{friston2010free} provides the mathematical frame for prediction error driven updates.

\paragraph{Action categorizer.}
A small classifier routes candidate actions to delegate, review, question, or notify. The category determines both the inbox affordance and the default cost of interruption budget.

\section{Prompt Templates}
\label{app: prompt}

We sketch four representative prompt templates. Concrete prompt engineering is beyond the scope of a position paper; the templates illustrate the structure each component requires.

\paragraph{P1, Cross context relevance assessor.}
Given the situational state $s_t$, a candidate action $a$, and recent dismissal or delegation history, produce \texttt{\{relevance\_score, urgency\_score, interrupt\_now: bool, rationale, suggested\_category\}}.

\paragraph{P2, Silence reasoner.}
Given a detected item that did not pass the threshold for showing a message, produce a one line \texttt{deferred\_summary} for the weekly digest.

\paragraph{P3, Action framer.}
Given a shown action and the chosen category, produce the inbox ready message: a one line headline, a three to five line context, and the affordances (delegate, review, question, notify).

\paragraph{P4, Preference update interpreter.}
Given a developer response (delegate, dismiss, defer, edit, ignore) and the latency, produce the implicit signal label used to update the developer model $\theta$.
